# Supplementary material for: Attentive Explanations: Justifying Decisions and Pointing to the Evidence (Extended Abstract)
Source: arXiv:1711.07373 source file (2017-11-17)
Supplement: Supplementary file 1 [file appendix.tex]

In this appendix material, we provide more details about our VQA model% and \cite{hendricks16eccv}, 
as well as additional qualitative results. In \autoref{sec:vqa_model}, we provide an evaluation of our proposed VQA model on the original VQA task, showing improved results. %while \autoref{sec:hendricks} details the differences of our model to \cite{hendricks16eccv}. 
In \autoref{supp:qualitative} we discuss our additional qualitative results in Figures \ref{fig:VQAqualitative}, \ref{fig:ACTqualitative}, \ref{fig:VQAqualitative-sameQA},  \ref{fig:VQAqualitative-sameimage}, and \ref{fig:ACTqualitative:similar:activity}.
%In this supplemental material we provide additional details to our models (see a more detailed visualization of our model in Figure~\ref{fig:model}) as well as qualitative and quantitative results. In \autoref{sec:vqa_model} we provide an evaluation of our proposed VQA model on the original VQA task, showing improved results while \autoref{sec:hendricks} details the differences of our model to \cite{hendricks16eccv}. In \autoref{sec:human:eval} we add a human evaluation of  our textual justifications, showing clear improvements over prior work \cite{hendricks16eccv}. Moreover, \autoref{sec:eval:attention} adds a quantitative evaluation of the pointing task on our collected human pointing data. The results indicate competitive performance of our attention maps compared to several baselines on multiple metrics. In \autoref{supp:qualitative} we discuss our additional qualitative results in Figures \ref{fig:VQAqualitative}, \ref{fig:ACTqualitative}, \ref{fig:VQAqualitative-sameQA},  \ref{fig:VQAqualitative-sameimage}, and \ref{fig:ACTqualitative:similar:activity}.

\section{Visual Question Answering Model}
\label{sec:vqa_model}
The VQA model that we use throughout the experiments is based on the state-of-the-art MCB model \cite{fukui16emnlp}, but trains and evaluates faster (reduction by about 30\%). The main difference between the two models is how they combine two different representations and create multi-modal features.

Our VQA model encodes the image with ResNet and the question with an LSTM, just as in the MCB model. However, instead of doing Compact Bilinear Pooling \cite{gao16cvpr} between the two representations, our model simply embeds the encoded image feature using $1\times1$ convolutions and applies element-wise multiplication between the embedding and the LSTM feature. Whereas the MCB model tries to create a rich multi-modal feature by approximating the outer product of two representations, our model tries to learn the proper alignment of the representations so that when merged with element-wise multiplication, it creates a feature that is as powerful as the MCB feature. This improved model leads to an increase of 0.5\% when training on the train set, and 0.8\% when training on train-val.

% \section{Comparison to  Hendricks \etal \cite{hendricks16eccv}}
% \label{sec:hendricks}
% In the main paper and in the following sections we compare to the results from Hendricks \etal \cite{hendricks16eccv} using their implementation, but the same feature representation as our approach.
% The differences of our explanation model and the explanation model of~\cite{hendricks16eccv} are as follows. \cite{hendricks16eccv} generates explanatory sentences by using ResNet features extracted from the entire image. Generated sentences are conditioned on both the image and class predictions. The explanations are trained with a discriminative loss which enforces the generated sentence to contain class-specific information. Additionally,~\cite{hendricks16eccv} is trained on descriptions.
% Our model on the other hand, has an integrated attention mechanism that is used to generate textual explanations as well as to point to the evidence of the explanation. We observe from~\autoref{tbl:generation_automatic_actX} of the main paper that in all metrics, our method outperforms \cite{hendricks16eccv}. Ours without attention is similar to~\cite{hendricks16eccv} in the sense that there is no attention mechanism, however, ours without attention does not use the discriminative loss and is also trained on explanations.

\begin{table}[tb]
\centering
\small
\begin{tabular}{l|rr}
\toprule
 \bf  &  \multicolumn{2}{c}{Training data} \\ 
 \bf Method &  Train & Train+Val \\ \cmidrule(lr){1-1}\cmidrule(lr){2-3}
MCB \cite{fukui16emnlp} & 62.5 & 64.2 \\
 Our VQA model & \bf{63.0} & \bf{64.8}\\
 \bottomrule
\end{tabular}
\caption{OpenEnded results on VQA dataset \cite{antol2015vqa}, test-dev. The columns indicate the accuracy of the model after being trained on train set and train+val set, respectively. Our model achieves slightly  higher accuracy and the previous VQA challenge winner MCB \cite{fukui16emnlp}}
\label{tab:VQA}
\end{table}

\begin{figure*}[h]
\begin{center}
  \includegraphics[width=\linewidth]{VQA_qualitative_sup}
\end{center}
\caption{VQA-X results. Figure on the left: We show various qualitative results with correctly predicted answer and observe that the explanation justifies the answer accordingly. Figure on the right: We show results with incorrectly predicted answer and observe that although the answer is incorrect, our model can provide visual and textual explanations on why the model might be failing in those cases.}
\label{fig:VQAqualitative}
\end{figure*}

\begin{figure*}[h]
\begin{center}
  \includegraphics[width=\linewidth]{ACT_qualitative_sup}
\end{center}
\caption{ACT-X results. Figure on the left: We show various qualitative results with correctly predicted answer and observe that the explanation justifies the answer accordingly. Figure on the right: We show results with incorrectly predicted answer and observe that although the answer is incorrect, our model can provide visual and textual explanations on why the model might be failing in those cases.}
\label{fig:ACTqualitative}
\end{figure*}

\begin{figure*}[h]
\begin{center}
  \includegraphics[width=\linewidth]{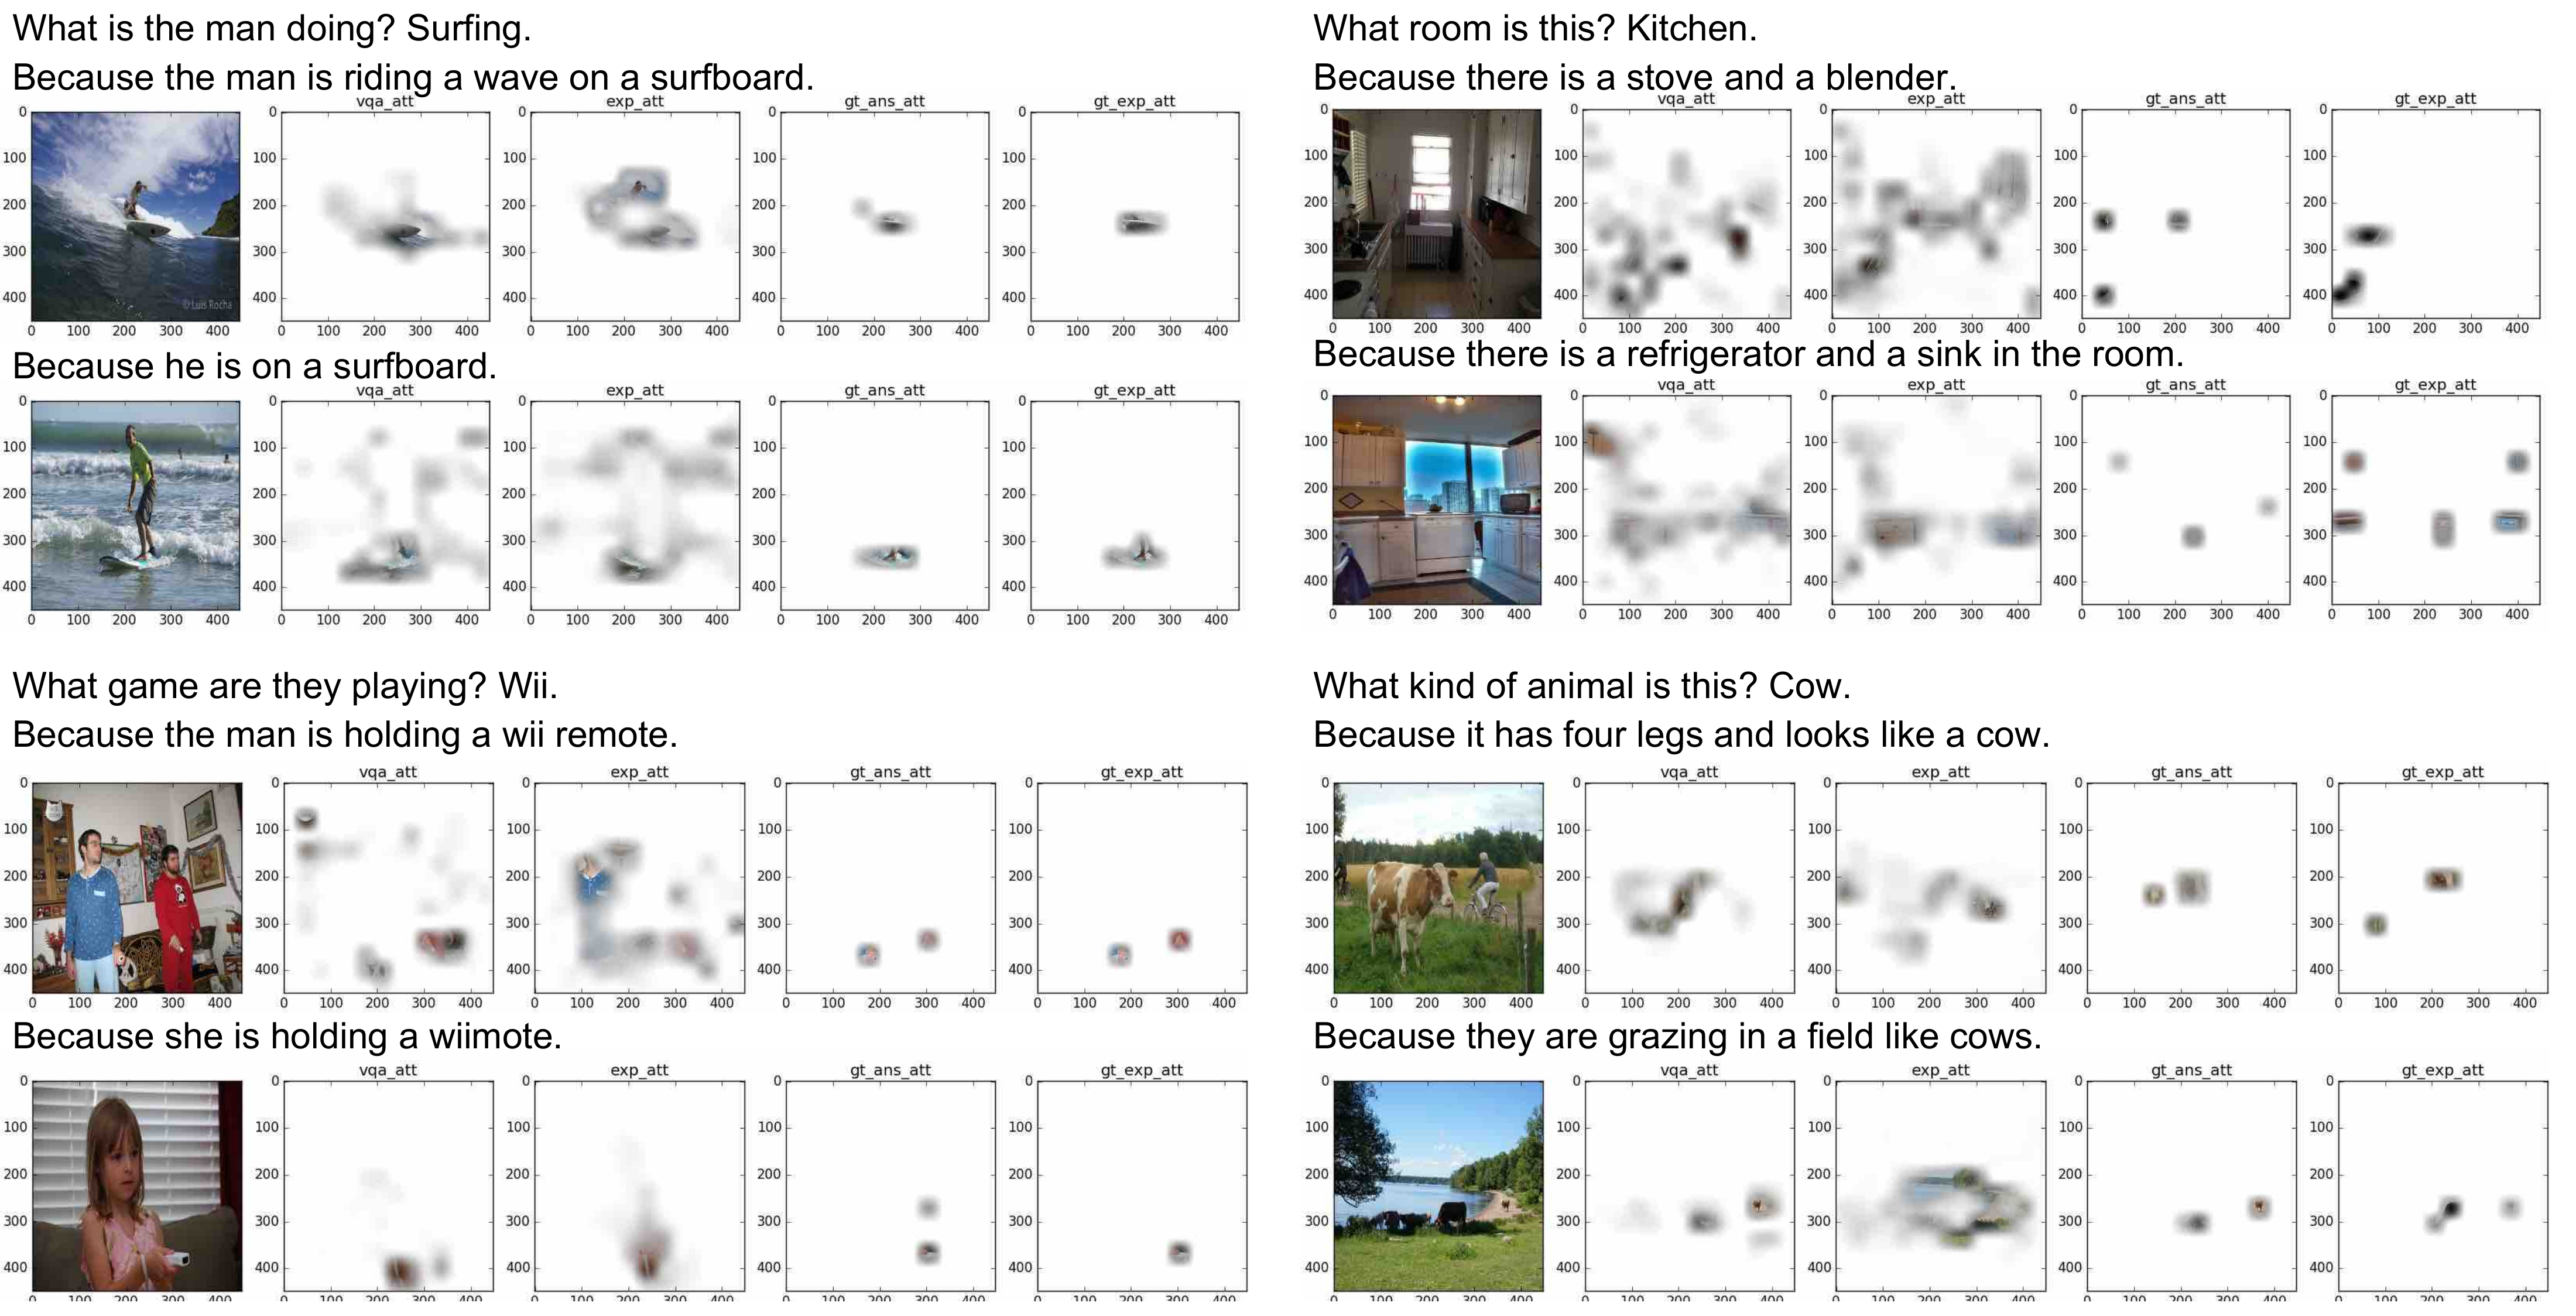}
\end{center}
\caption{VQA-X results with the same question/answer pair. We select results with the same question and answer pair with two different images and show that although the QA pairs are the same, for different images our model generates different explanations. (Answers are correctly predicted)}
\label{fig:VQAqualitative-sameQA}
\end{figure*}

\begin{figure*}[h]
\begin{center}
  \includegraphics[width=\linewidth]{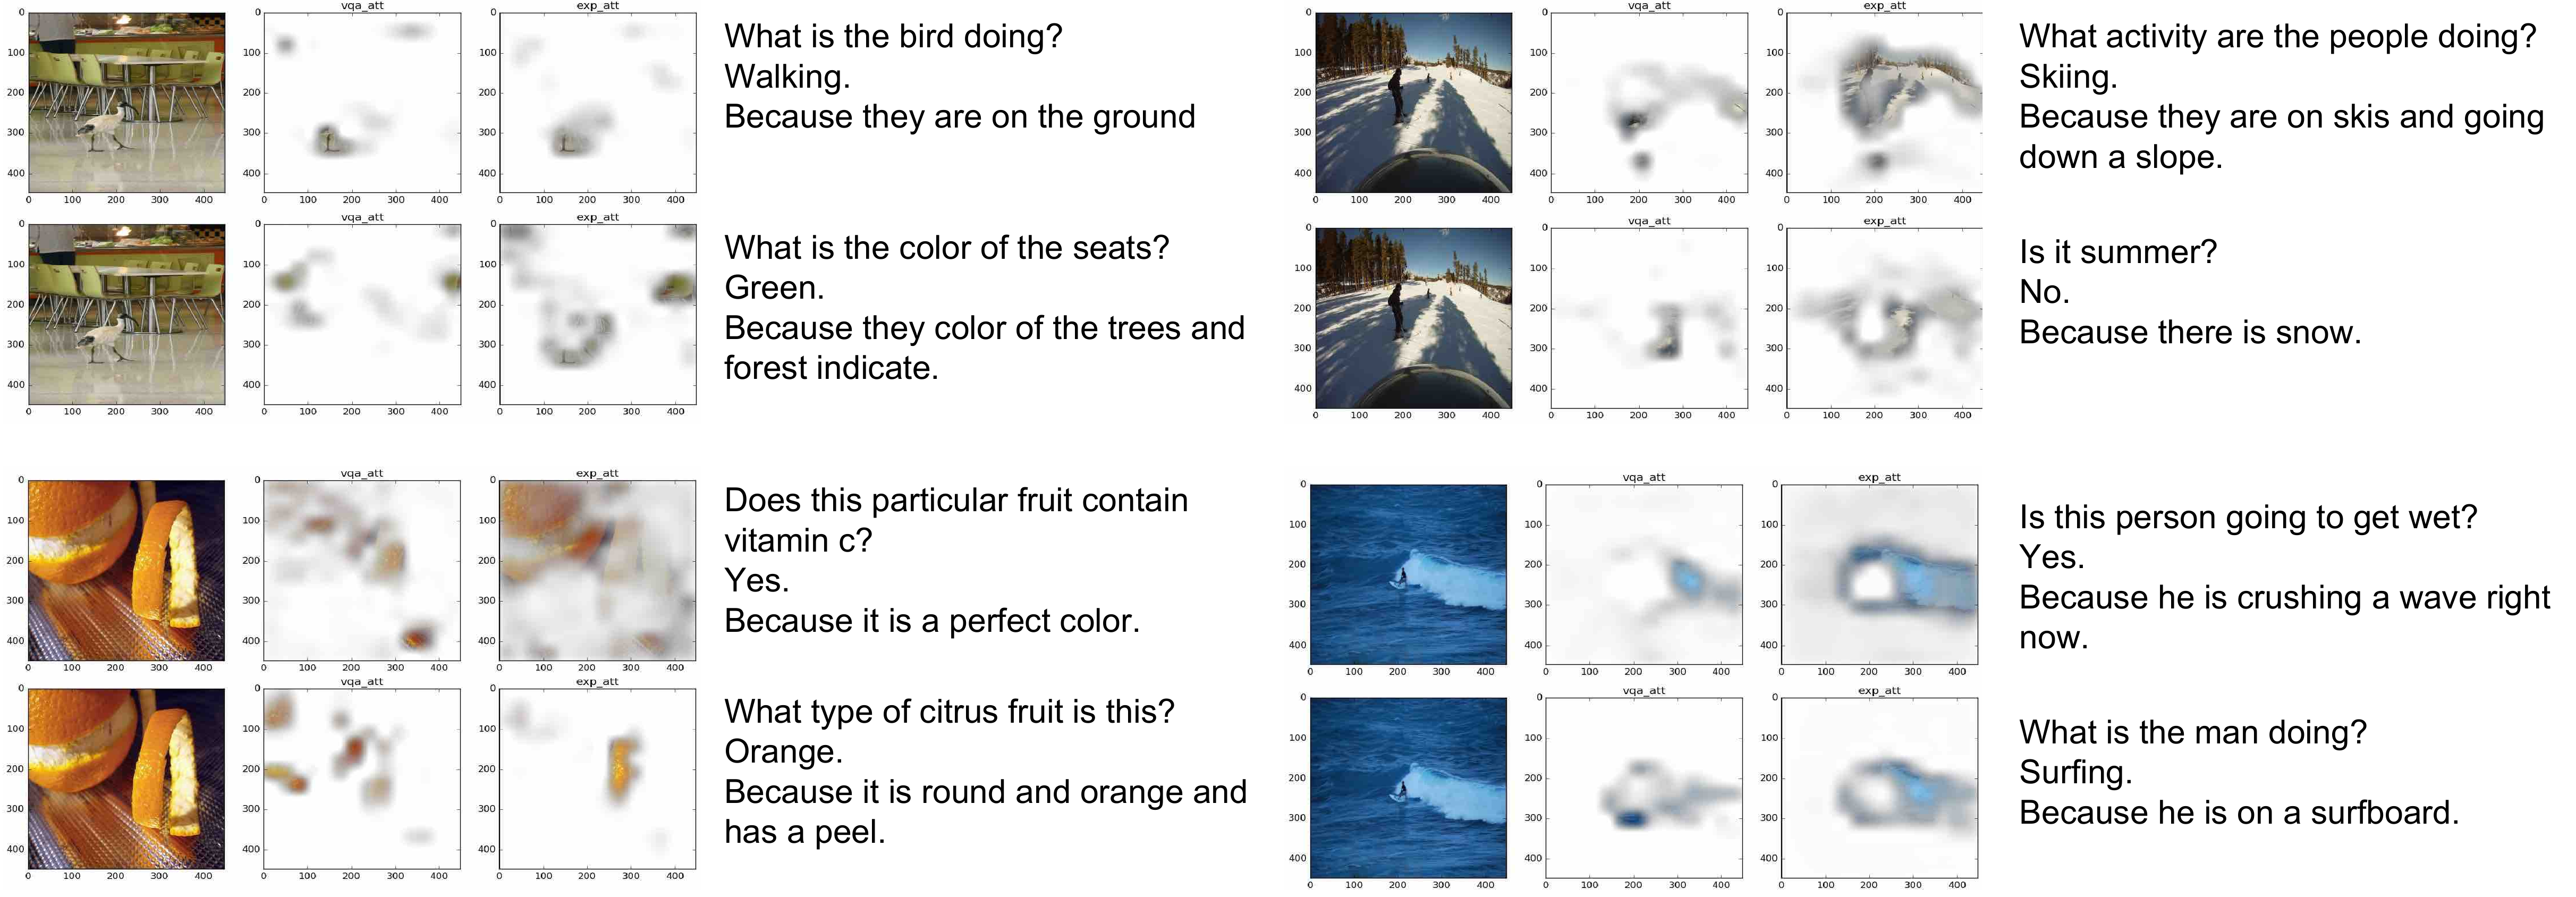}
\end{center}
\caption{VQA-X results with same image and different questions. We select results with the same image and different Q/A pairs and show that although the images are the same, our model is able to answer the questions differently and generate a different explanation accordingly. (Answers are correctly predicted)}
\label{fig:VQAqualitative-sameimage}
\end{figure*}

\begin{figure*}[h]
\begin{center}
  \includegraphics[width=\linewidth]{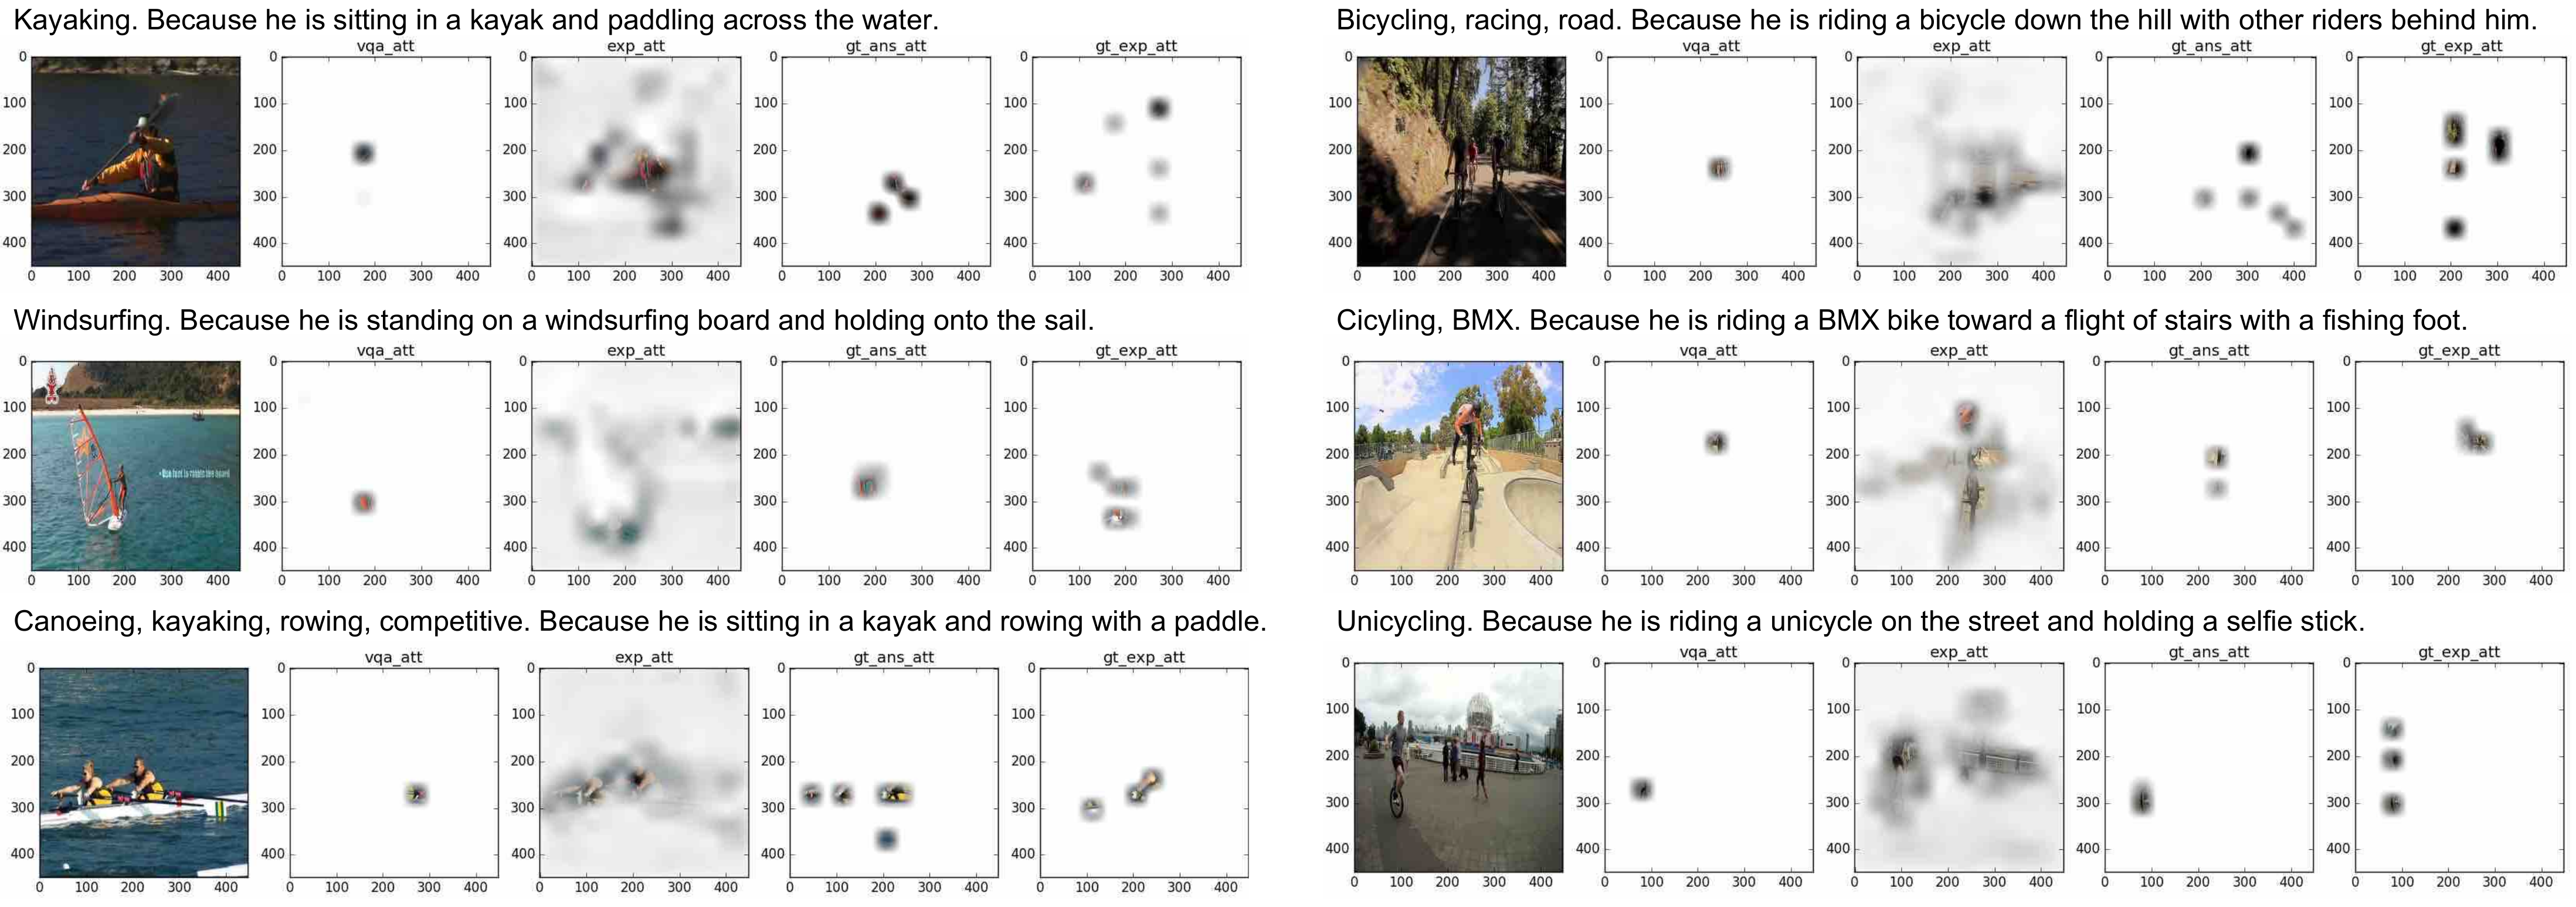}
\end{center}
\caption{ACT-X results with similar activities. Figure on the left: We show results with fine-grained activities all related to sailing, canoeing, kayaking and observe that both the fine-grained activities are correctly predicted and the explanations match the activity and the image. Figure on the right: We show results with fine-grained activities all related to bicycling and observe that both the fine-grained activities are correctly predicted and the explanations match the activity and the image.}
\label{fig:ACTqualitative:similar:activity}
\end{figure*}

\section{Qualitative Results}
\label{supp:qualitative}

Figures \ref{fig:VQAqualitative}, \ref{fig:ACTqualitative}, \ref{fig:VQAqualitative-sameQA},  \ref{fig:VQAqualitative-sameimage}, and \ref{fig:ACTqualitative:similar:activity} show additional qualitative results on our proposed datasets.
Figures \ref{fig:VQAqualitative} and \ref{fig:ACTqualitative} compare explanations when the answer or action label are correctly and incorrectly predicted.
In addition to providing an intuition about why predictions are correct, our explanations frequently justify why the model makes incorrect predictions. 
For example, when incorrectly predicting whether one should stop or go (Figure  \ref{fig:VQAqualitative}, second row, right), the model outputs ``Because the light is green'' suggesting that the model has mistaken a red light for a green light, and furthermore, that green lights mean ``go''.
When asked ``What is the person doing?'' (Figure  \ref{fig:VQAqualitative}, bottom row, right), the model incorrectly predicts ``playing tennis''.  Though this prediction is incorrect, the explanation ``Because he is holding a tennis racket'' suggests what visual elements could have confused the VQA model.
Figure \ref{fig:ACTqualitative} shows similar trends on the ACT-X dataset. 
For example, when incorrectly predicting the activity bicycling for an image depicting motor scooter, the explanation ``Because he is riding a bicycle down a road with other riders behind him'' suggests that the motor scooter may have been misclassified as a bicycle.
We reiterate that our model \emph{justifies} predictions and does not fully explain the inner-workings of deep architectures.
However, these justifications demonstrate that our model can output intuitive explanations which could help those unfamiliar with deep architectures make sense of model predictions.

Figures \ref{fig:VQAqualitative-sameQA} and \ref{fig:VQAqualitative-sameimage} demonstrate that both images and the question/answer pair are needed for good explanations.
Figure \ref{fig:VQAqualitative-sameQA} shows explanations for different images, but with the same question/answer pair.
Importantly, explanation text and visualizations change to reflect image content.
Figure  \ref{fig:VQAqualitative-sameimage} shows that when different questions are asked about the same images, explanations provide information which are specific to the questions.

Figure \ref{fig:ACTqualitative:similar:activity} shows that explanations on the ACT-X dataset discuss small details important for differentiating between similar classes.  For example, when explaining kayaking and windsurfing, it is important to mention the correct sporting equipment instead of image context.  
